# Supplementary material for: State Diagram of the Non-Reciprocal Cahn-Hilliard Model and the Effects of Symmetry
Source: arXiv:2503.07579 source file (2025-12-23)
Supplement: Supplementary file 1 [file supp.pdf]

# Phase diagram of the Non-Reciprocal Cahn-Hilliard model and the effects of symmetry

## Supplementary Material

Martin Kjøllesdal Johnsrud 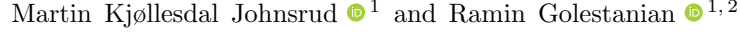<sup>1</sup> and Ramin Golestanian 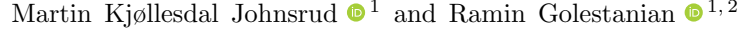<sup>1, 2</sup>

<sup>1</sup>*Max Planck Institute for Dynamics and Self-Organization (MPI-DS), D-37077 Göttingen, Germany*

<sup>2</sup>*Rudolf Peierls Centre for Theoretical Physics, University of Oxford, Oxford OX1 3PU, United Kingdom*

(Dated: March 10, 2025)

### I. ADDITIONAL FIGURES

We have included pictures of the full 3D phase diagrams from additional angles. Figure S1 shows the SO(2) model, and Figure S2 the C<sub>4</sub> model. To illustrate where the cuts in Figure 2 in the main text are done, we include inserting them into the 3D. This is shown in Figure S3. The subplots are arranged as in the main text. In the case of the C<sub>4</sub> model, there are two more scalings of the phase diagrams not shown in the main text. All parameters may be scaled by  $\sqrt{u\bar{\varphi}_1}$ , in which case the correlation lengths take the form

$$\kappa'_{\pm} = r' + 3 \left( 1 + v_1'^2 \right) \pm \sqrt{9 \left( 1 - v_1'^2 \right)^2 - \alpha'^2}, \quad (\text{S1})$$

where primes indicate re-scaled parameters, and scaling by  $\alpha$ , which gives

$$\kappa''_{\pm} = r'' + 3 \left( v_1''^2 + v_2''^2 \right) \pm \sqrt{9 \left( v_1''^2 - v_2''^2 \right)^2 - 1}. \quad (\text{S2})$$

These scalings give two new 3D phase diagrams, and two new sets of 2D slices of these 3D shapes. These are shown in Figure S4.

### II. VIDEOS

There are three videos included as supplementary material, referenced in the main text. Table I gives an overview of the videos, and their parameter values. All simulations used a time step of  $\Delta t = 1.6 \cdot 10^{-5}$ .

TABLE I. The videos included as supplemental material, and the parameter values used to generate them.

| Video nr. | $u, -r$ | $\alpha$ | $D$                | $\bar{\varphi}_1$ | $\bar{\varphi}_2$ |
|-----------|---------|----------|--------------------|-------------------|-------------------|
| 1         | 10      | 2        | $2 \times 10^{-4}$ | -0.2              | -0.1              |
| 2         | 10      | 1        | $1 \times 10^{-5}$ | -0.2              | 0                 |
| 3         | 40      | 0        | $2 \times 10^{-4}$ | -0.8              | 0                 |

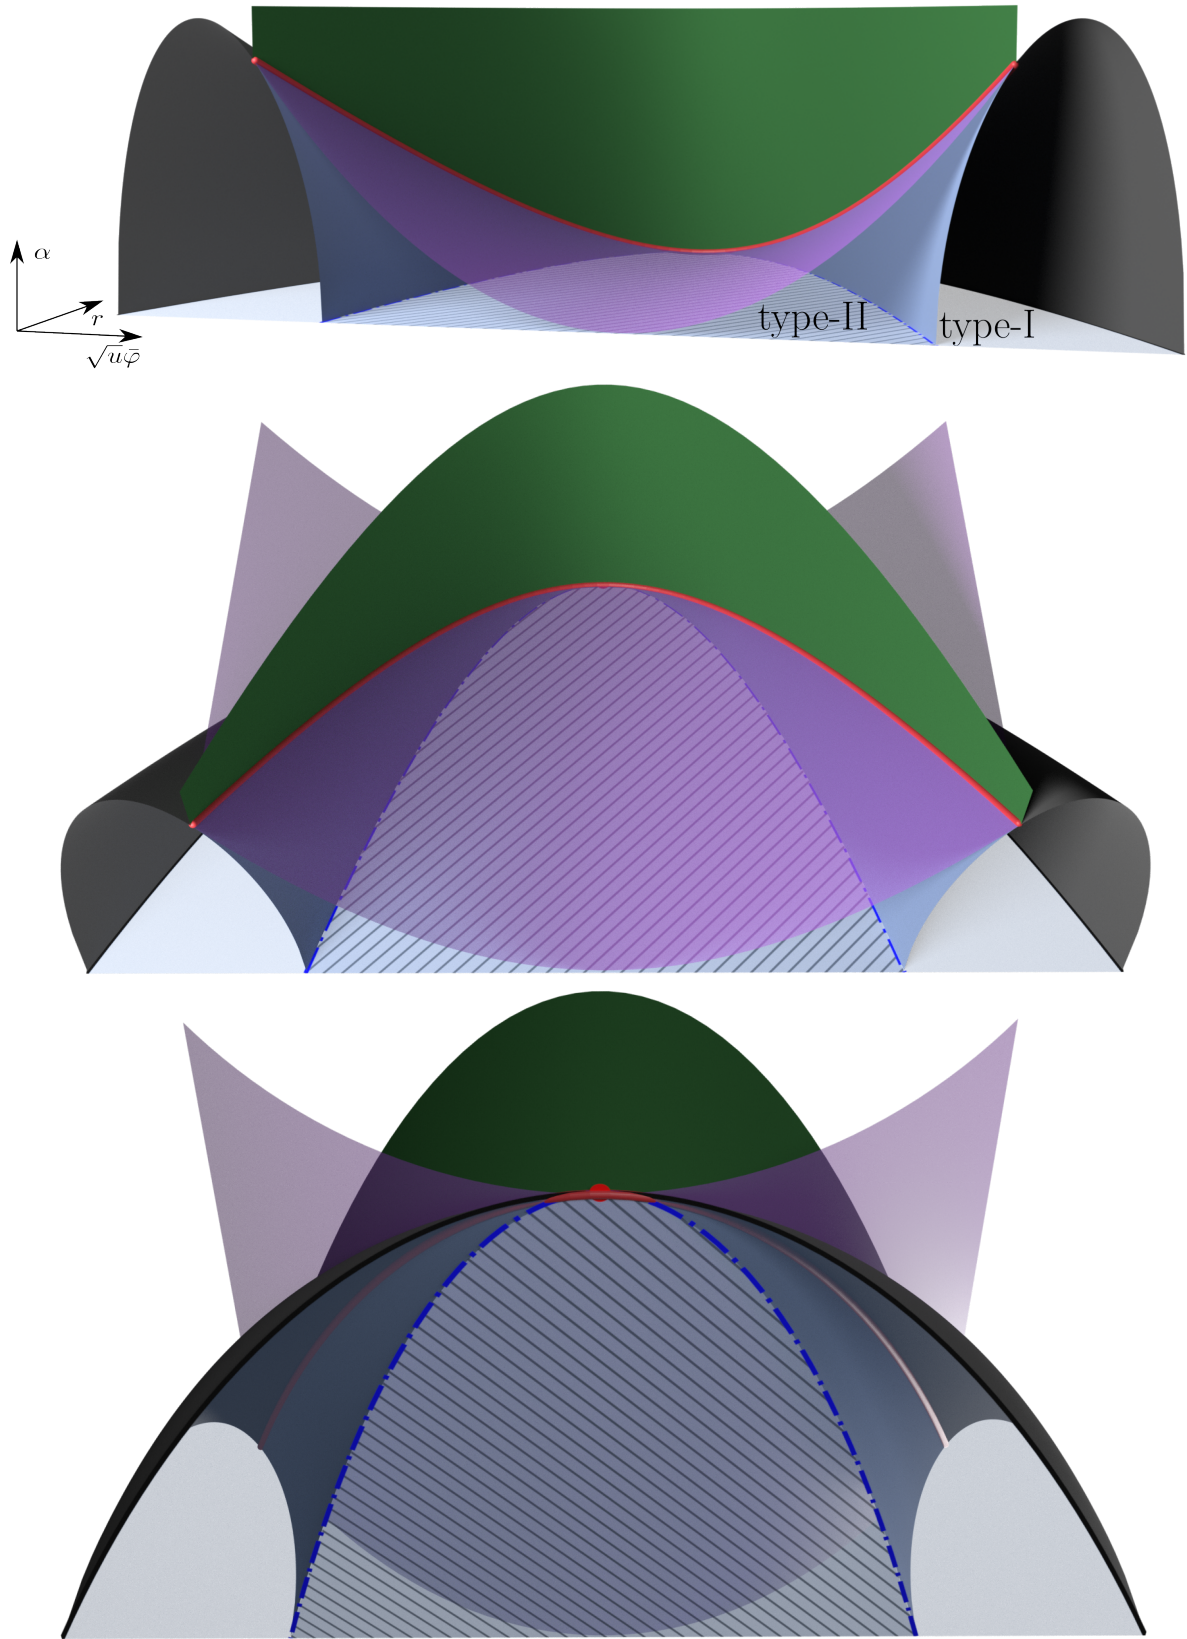

FIG. S1. The linear phase diagram of the SO(2) model.

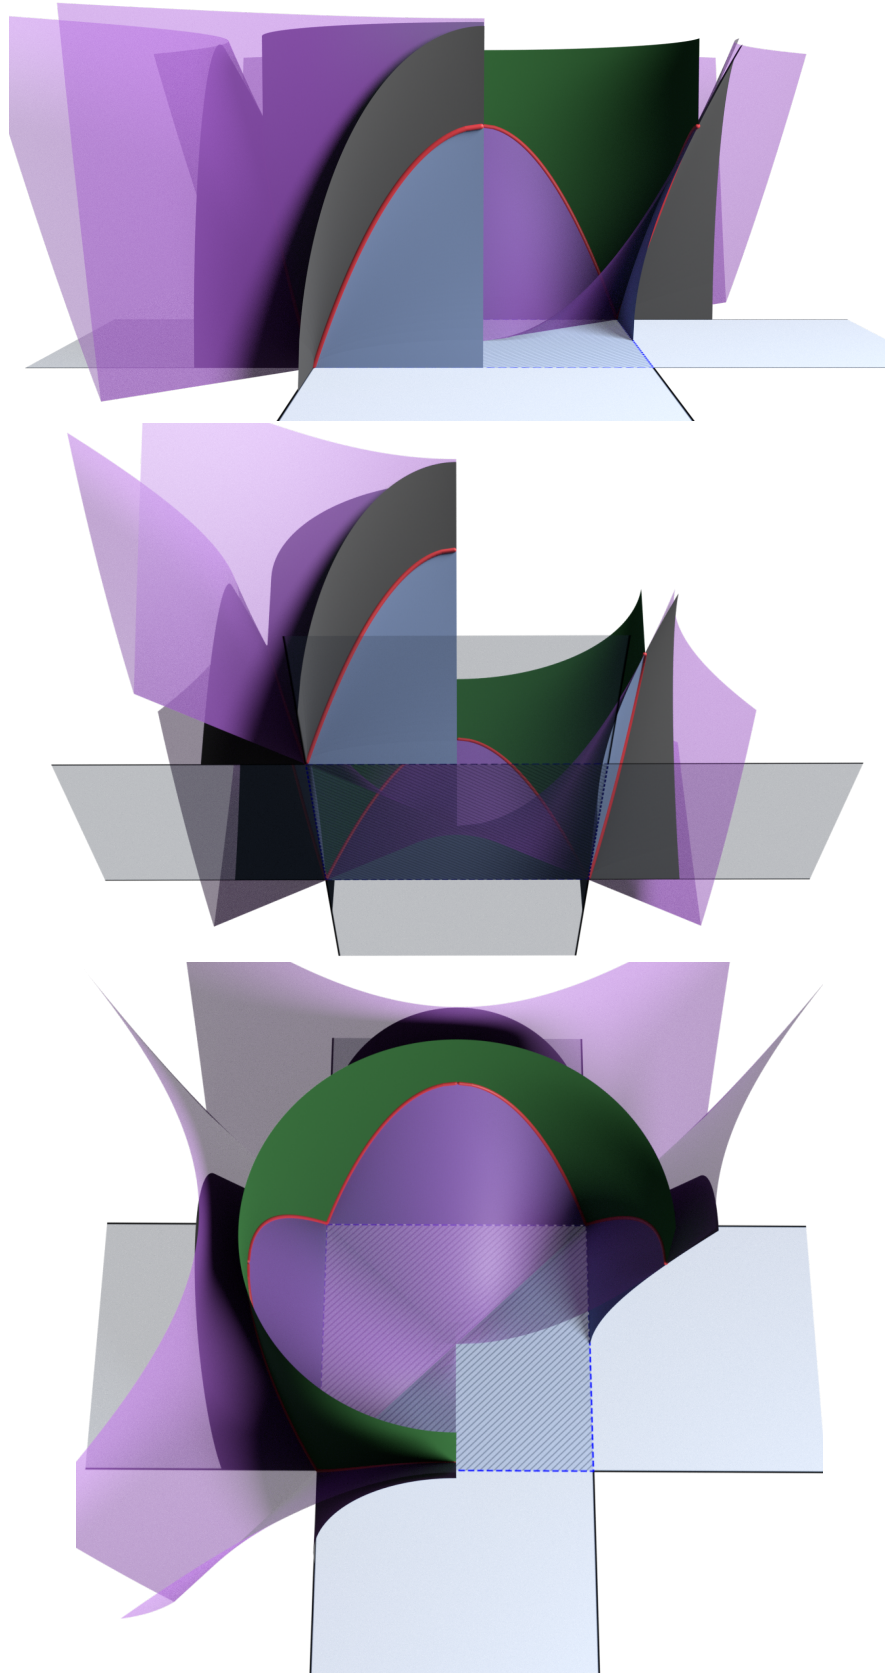

FIG. S2. The linear phase diagram of the  $C_4$  model.



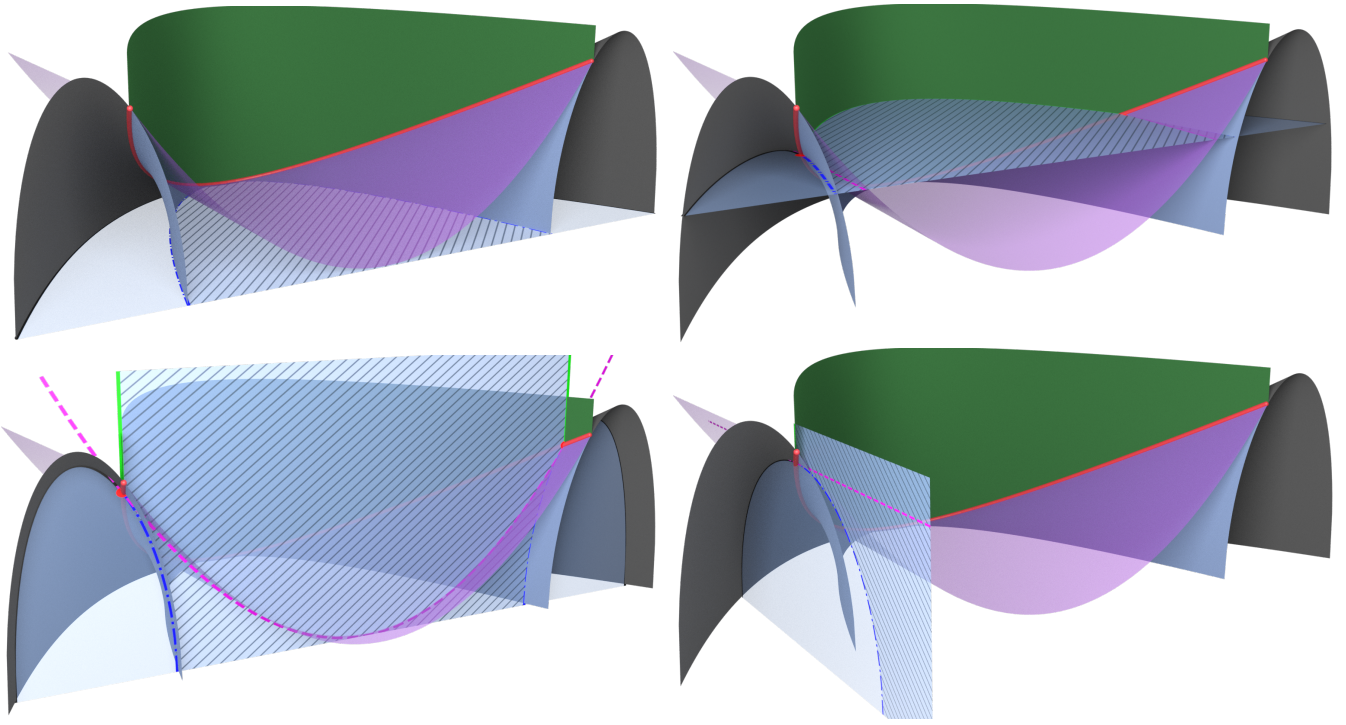

FIG. S3. The cuts into the phase are placed in the full 3-dimensional diagram of the SO(3) model.

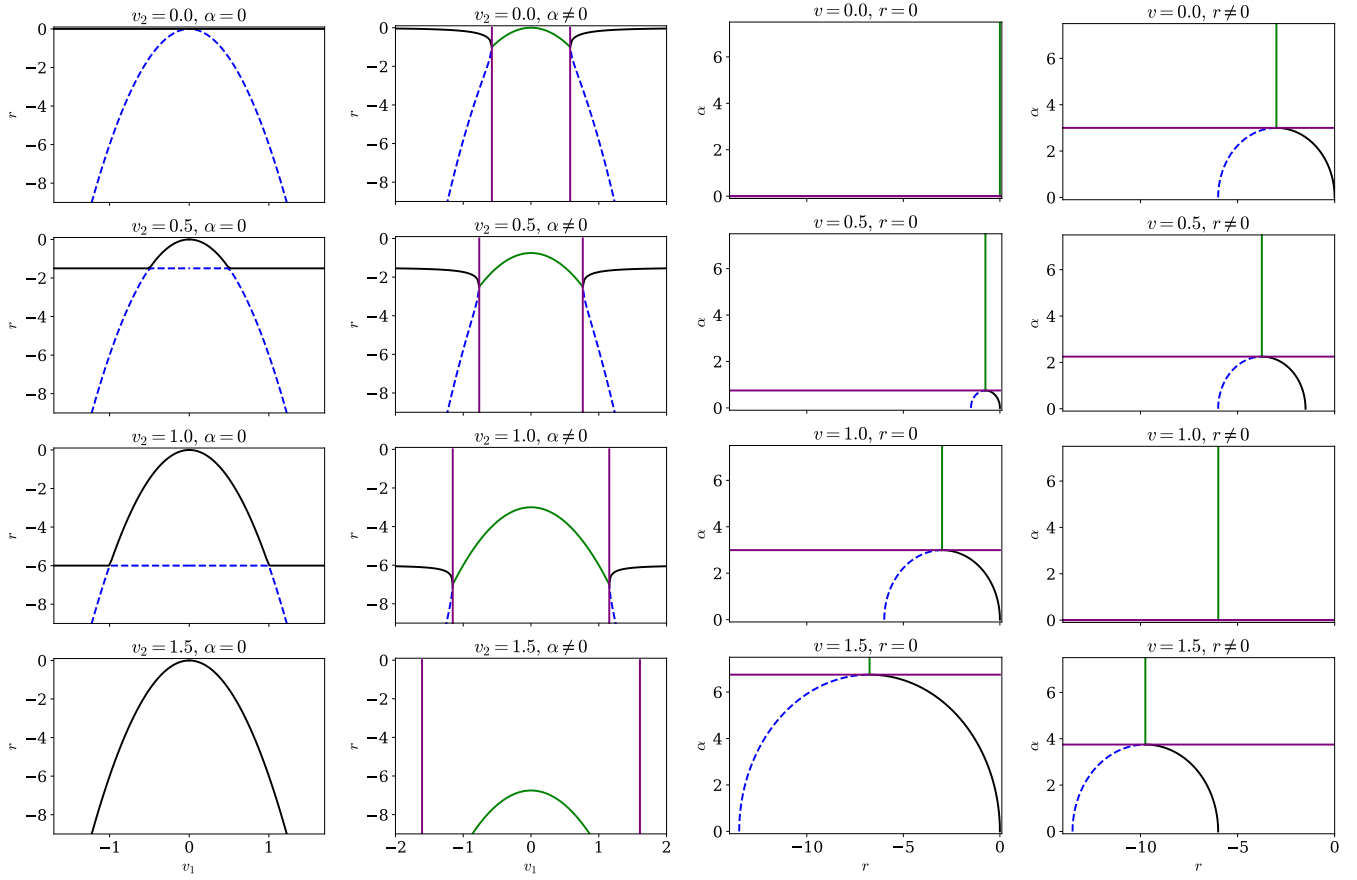

FIG. S4. The phase diagrams, scaled by  $\alpha$  (left) and  $v_2$  (right).
